# Supplementary material for: A Noisy-Label-Learning Formulation for Immune Repertoire Classification and Disease-Associated Immune Receptor Sequence Identification
Source: arXiv:2307.15934 source file (2023-07-29)
Supplement: Supplementary file 1 [file appendix.tex]

\begin{table*}[!h]
     \centering
     \resizebox{\textwidth}{!}{ %   
     \begin{tabular}{lll|lll|lll}
         \toprule
 		 index & sequence & conf. & index & sequence & conf. & index & sequence & conf. \\ \midrule
 		 1 & CASSPARNTEAFF & 0.69 &2 & CASSPTRNTEAFF & 0.69 &3 & CASSRLAASTDTQYF & 0.68 \\
         4 & CASSPQRNTEAFF & 0.68 &5 & CASSPYRNTEAFF & 0.68 &6 & CASSRLAGGTDTQYF & 0.67 \\
         7 & CASSPSRNTEAFF & 0.67 &8 & CASSLSWGGFYNEQFF & 0.67 &9 & CASSLIGVSSYNEQFF & 0.66 \\
         10 & CASSLQGYSNQPQHF & 0.66 &11 & CASSQDWGDGYTF & 0.66 &12 & CATSRGTVSYEQYF & 0.65 \\
         13 & CASSLTSEQFF & 0.64 &14 & CASSPRWQETQYF & 0.64 &15 & CASSVLAGPTDTQYF & 0.64 \\
         16 & CASSLGGAGDTQYF & 0.64 &17 & CASSSAYYGYTF & 0.63 &18 & CASSSQTGTIYGYTF & 0.63 \\
         19 & CASTPGDEQFF & 0.63 &20 & CASSLRGTDYEQYF & 0.63 &21 & CASSLGDRAYNEQFF & 0.63 \\
         22 & CASSFGVNTEAFF & 0.63 &23 & CASNRDRGRYEQYF & 0.63 &24 & CASSVVNEQFF & 0.63 \\
         25 & CATFDGNTGELFF & 0.62 &26 & CATSDGDTQYF & 0.62 &27 & CASSLGDRPDTQYF & 0.62 \\
         28 & CASSGLNEQFF & 0.62 &29 & CASSYSSGELFF & 0.61 &30 & CASSLSPSTGNYGYTF & 0.61 \\
         31 & CASSRDRNYGYTF & 0.61 &32 & CASSVTGGTDTQYF & 0.60 &33 & CASSHRDRNYEQYF & 0.60 \\
         34 & CASSLLWDQPQHF & 0.60 &35 & CASSIGPLEHNEQFF & 0.60 &36 & CASSLAPGATNEKLFF & 0.59 \\
         37 & CATHSGNTGELFF & 0.59 &38 & CATSRVAGETQYF & 0.58 &39 & CASTQGLAGLTDTQYF & 0.58 \\
         40 & CASSLEGYTEAFF & 0.56 &41 & CASSSVNEQFF & 0.55 &42 & CASSLGLNYEQYF & 0.51 \\
         43 & CATSDDRDTGELFF & 0.41 &44 & CASSPGDEQYF & 0.38 &45 & CAWSVSDLAKNIQYF & 0.35 \\
         46 & CASRPTGYEQYF & 0.13 &47 & CASSSGTGPNEKLFF & 0.13 &48 & CASSWDRGTEAFF & 0.13 \\
         49 & CASSLVGDGYTF & 0.11 &50 & CASSLDSIASGNTIYF & 0.08 & \\ \bottomrule
     \end{tabular}
     }
     \caption{List of CMV-associated sequences in the CMV dataset that previously identified through \textit{in vitro} experiments and our model's confidence.
     Our model, without using any sequence-level association information during training, assigns a larger part of them more than 50\% probability of being CMV-associated.
}
    \label{high_conf_seq}
\end{table*}

\begin{table*}[!h]
     \centering
     \resizebox{\textwidth}{!}{ %   
     \begin{tabular}{lll|lll|lll}
         \toprule
 		 index & sequence & conf. & index & sequence & conf. & index & sequence & conf. \\ \midrule
 		 1 & CASSQSQLRTEAFF & 0.99 &2 & CASSFPSRDPIF & 0.99 &3 & CASSLGQSTDTQYF & 0.99 \\
         4 & CASSSPFRQTEAFF & 0.99 &5 & CASSQDSSGGIPEQYF & 0.99 &6 & CASSELQGEVYEQYF & 0.99 \\
         7 & CASSQPVQGRPEAFF & 0.99 &8 & CATLEGVTGYTF & 0.99 &9 & CASSPRADTQYF & 0.86 \\
         10 & CASSSHDRQGTGSPLHF & 0.82 &11 & CASGLVIGHGQETQYF & 0.82 &12 & CSASPGQGYTF & 0.81 \\
         13 & CASSSAEQGSYEQYF & 0.81 &14 & CASSLAGPERSSNQPQHF & 0.81 &15 & CASSPQGLEETQYF & 0.80 \\
         16 & CASSSHDFEGVLSPLHF & 0.80 &17 & CASSVQGGTYEQYF & 0.76 &18 & CASSRPNTEAFF & 0.73 \\
         19 & CASSSRGPEEQYF & 0.73 &20 & CASSSLAGGPASYNEQFF & 0.73 &21 & CATTLSSNSGNTIYF & 0.73 \\
         22 & CASSTSGGYEQYF & 0.73 &23 & CASTITGSTLEQYF & 0.73 &24 & CASSRLAGGVSEQYF & 0.73 \\
         25 & CASSRLAGGTGELFF & 0.72 &26 & CASSQDRRGGAFF & 0.72 &27 & CASSETGGTYEQYF & 0.72 \\
         28 & CASSLPQVPTEAFF & 0.72 &29 & CASSEGGLAGGLASTDTQYF & 0.71 &30 & CASSLEGLPLSNYGYTF & 0.71 \\
         31 & CASSPVGGDYEQYF & 0.71 &32 & CASSDADRDYTF & 0.70 &33 & CASSLTGQIYEQYF & 0.70 \\
         34 & CASRGGSSYEQYF & 0.70 &35 & CASSLASGYTF & 0.70 &36 & CASSSATGTVYGYTF & 0.70 \\
         37 & CASSLASQRTKRTQYF & 0.70 &38 & CASTGGSQPQHF & 0.70 &39 & CASGGTAVGDGYTF & 0.70 \\
         40 & CASSQYRADGYTF & 0.70 &41 & CASSGREVAPSEQFF & 0.70 &42 & CASSRTSATGELFF & 0.70 \\
         43 & CASTRTAGVYGYTF & 0.70 & &&\\ \bottomrule
     \end{tabular}
     }
     \caption{List of sequences in the CMV dataset that our model assigns high confidence (>0.7) but may haven't identified by previous studies.
     We report these for future experimental verification.}
    \label{ass_seq_conf}
\end{table*}
% \section{Associated sequences identification}
% We report our model's confidence on the know CMV-associated sequences in Table \ref{ass_seq_conf}.  
% We also report some confident sequences for future experimental verification in Table \ref{high_conf_seq}.
